# Supplementary material for: High-accuracy mesh-free quadrature for trimmed parametric surfaces and volumes
Source: arXiv:2101.06497 source file (2022-01-02)
Supplement: Supplementary file 1 [file appendixC_momentFitting.tex]

\section{Moment Fitting}
\label{app:momentFitting}
The \spectral\ and \spectralPE\ algorithms described in Section~\ref{sec:algorithm} can also be used as an input to moment fitting, through which interiority of the quadrature points can be achieved. Moment fitting is a technique that was reintroduced to the engineering community in \cite{mousavi2010generalized}. In moment fitting, a linear system of equations of the form
\begin{equation*}
\begin{bmatrix} 1 & 1 & 1 &\ldots & 1\\
 x_1 & x_2 & x_3 &\ldots & x_n \\
 y_1 & y_2 & y_3 &\ldots & y_n \\
 x_1^2 & x_2^2 & x_3^2 &\ldots & x_n^2\\
 x_1y_1 & x_2y_2 & x_3y_3 & \ldots &  x_ny_n\\ 
 y_1^2 & y_2^2 & y_3^2& \ldots & y_n^2\\
\vdots & \vdots & \vdots & \ddots & \vdots \\
\end{bmatrix}\begin{bmatrix} w_1 \\ w_2\\ w_3 \\\vdots \\ w_n \end{bmatrix} = \begin{bmatrix}
\int_D 1 dA\\
\int_D x dA\\
\int_D y dA\\
\int_D x^2 dA\\
\int_D xy dA\\
\int_D y^2 dA,\\
\vdots\\
\end{bmatrix}
\end{equation*}
is used to find corresponding quadrature weights $\{w_i\}_{i=1}^n$ for a given pre-specified set of quadrature points $\{ (x_i,y_i)\}_{i=1}^n$ for integrating over a region $D$. The number of quadrature points $n$ is typically taken to be much larger than the number of monomials fitted. The quadrature points $\{ (x_i,y_i)\}_{i=1}^n$ can be specified to be within the domain of integration $D$ \cite{thiagarajan2018shape}. However, the quadrature points should be chosen with care, as their locations impact the accuracy and stability of the resulting quadrature scheme for general integrands. Note that non-negative quadrature weights can be ensured through the solution of a related constrained optimization problem \cite{keshavarzzadeh2018numerical}.

Our method can obtain exact results for the right-hand side vector for rational domains $D$, eliminating any error in the moment-fitting procedure stemming from monomial integration and making it a prime candidate for evaluating the right-hand side. Moreover, the lack of a guarantee of interiority of quadrature points in our method is one of its potential disadvantages, so using it with moment-fitting can be helpful in contexts when interiority is needed. We leave exploration of such a method to a future work.
