# Supplementary material for: High-accuracy mesh-free quadrature for trimmed parametric surfaces and volumes
Source: arXiv:2101.06497 source file (2022-01-02)
Supplement: Supplementary file 2 [file appendixD_circle_example.tex]

\section{Detailed, Step-by-step Application of the \spectralPE\ Algorithm over a Circle}
\label{app:detailed_example}
In this section, we describe the steps of the \spectralPE\ algorithm in detail for the integral $\int_\Omega xy^2 dxdy$, where $\Omega$ is the circular region defined in Section~\ref{sec:circle_def} with center $(x_0,y_0) = (0,0)$ and radius $1$. The steps in this section are visualized in Figure~\ref{fig:overview} and the final quadrature rule produced is shown in Figure~\ref{fig:quadrature_points_circle}. Note that the maximum polynomial degree of the integrand is $k=3$. As described in Section~\ref{sec:algorithm}, the \spectralPE\ algorithm for computing polynomially-exact quadrature rules proceeds for each component curve $\mathbf{c}_i$ in two steps: \begin{enumerate}[(1)]
  \item Compute a set of intermediate quadrature points and weights for the Green's Theorem line integral corresponding to $\mathbf{c}_i$ and
  \item Compute quadrature rules to exactly evaluate the antiderivative function numerically at each intermediate quadrature point.
\end{enumerate} 

Let us first consider the curve $\mathbf{c}_0$, noting that the following procedure must be applied to each of the $\{\mathbf{c}_i\}_{i=0}^3$. We have
\begin{equation*}
\mathbf{c}_0 = \begin{cases} x_0(s) = \left( \frac{(1-s)^2 + \sqrt{2} (1-s)s}{(1-s)^2 +  \sqrt{2} (1-s)s + s^2} \right) = \left( \frac{1+(\sqrt{2}-2)s + (1-\sqrt{2})s^2}{ 1+(\sqrt{2}-2)s + (2-\sqrt{2})s^2} \right)\\
y_0(s) = \left(\frac{\sqrt{2} (1-s)s + s^2}{(1-s)^2 +  \sqrt{2} (1-s)s + s^2}\right) = \left( \frac{\sqrt{2}s + (1-\sqrt{2})s^2}{1+(\sqrt{2}-2)s + (2-\sqrt{2})s^2} \right).\end{cases}
\end{equation*} For the \spectralPE\ algorithm, the intermediate quadrature rule must be exact for the intermediate rational function appearing in the Green's theorem line integral in Equation~$\eqref{eq:green_par}$. In the actual algorithm, the antiderivative and the partial derivative terms are computed numerically. However, for demonstration purposes, we show the Green's theorem line integral for this curve and integrand with analytic antiderivative and partial derivative terms:
\begin{align*}
&\int_{\mathbf{c}_i} A_f(x(s),y(s))\frac{d x_i}{ds} ds = \int_0^1 \frac{1}{3}x_i(s) y_i(s) ^3 \frac{d x_i(s)}{ds} ds\\
= \int_0^1 \frac{1}{3} &\left( \frac{p(s)}{\left( 1+(\sqrt{2}-2)s + (2-\sqrt{2})s^2\right)^6} \right)ds,
\end{align*}
where $p(s)$ is a polynomial of degree $10$ which is too long to write out here, but is not important. Importantly, the integrand function has the same poles as the original Bernstein-\bezier\ curve, but with multiplicities multiplied by $k+3=6$. The next step in the algorithm is therefore to find these poles. In general, we use a numerical routine described in Sections~\ref{subsec:poles}~and~\ref{sec:conversion}. In this explanatory example, we find them analytically for demonstration purposes as
\begin{equation*}
p_{0,0} = \frac{1}{2} +\frac{\sqrt{2}}{4- 2\sqrt{2}}i,\hspace{.5cm}  p_{0,1} = \frac{1}{2} -\frac{\sqrt{2}}{4- 2\sqrt{2}}i.
\end{equation*} 
Finally, the rational functions which must be integrated exactly are those functions with poles $p_{0,0}$, $p_{0,1}$ each having multiplicity up to $6$. In general, we use the \textit{rfejer} routine to calculate the quadrature nodes and weights \cite{deckers2017algorithm}. In this case, there will be $13$ quadrature nodes and weights which exactly integrate this class of rational functions.

In the above derivation, we computed the partial derivative and antiderivative terms analytically. In general, these are not known analytically. Therefore, we generally numerically evaluate each of these as needed for each intermediate quadrature point. For example, the first intermediate quadrature point for $\mathbf{c}_0$ is $s_{0,0}= 0.004210269296207$ with weight $\gamma_{0,0} = 0.014622491933143$. In order to find the full quadrature rule, we must evaluate both the antiderivative and derivative terms at this point. 

For the antiderivative computation, we pick $C=-1$, because the lowest control point defining the entire domain has $y$-coordinate $-1$:
\begin{equation*}
A_f(x(s_{0,0}),y(s_{0,0}))=\int_{-1}^{y(s_{0,0})} f(x(s_{0,0}),t)dt.
\end{equation*}
This will cause the resulting final quadrature points for this intermediate quadrature point to be spread between $y=-1$ and $y=y(s_{0,0})$. To further clarify the effect of picking a particular $C$ value on the locations of the quadrature points, compare the quadrature points for the orange upper-right curve in Figure~\ref{fig:overview}, for which we took $C=-1$, to the quadrature points in Figure~\ref{fig:quadrature_points_circle}, in which we took $C=0$.	

  Because we know $f(x,y)$ is a polynomial of degree $3$, the number of Gaussian quadrature points necessary for exactness is $2$. The points and weights for the antiderivative quadrature rule for $s_{0,0}$ are
\begin{align*}
x_{0,0,0} &= \phantom{-}0.005961518538852,\hspace{.5cm}  x_{0,0,1} = \phantom{-}0.005961518538852,\\
y_{0,0,0} &= -0.577354024434498, \hspace{.5cm} y_{0,0,1} = \phantom{-}0.577336254424967,\\
\gamma_{0,0,0} &= \phantom{-}0.502980759269426, \hspace{.5cm} \gamma_{0,0,1} = \phantom{-}	0.502980759269426.
\end{align*}

The derivative at $s_{0,0}=0.008451616990154$ can also be evaluated numerically via deCasteljau's algorithm as $\frac{dx_0(s_{0,0})}{ds} = 1.417670137190716$. Therefore, the final quadrature weights for the two quadrature points, $(x_{0,0,0}, y_{0,0,0})$ and $(x_{0,0,1}, y_{0,0,1})$ are, respectively,  
\begin{align*}
w_{0,0,0} &= \gamma_{0,0}\gamma_{0,0,0}\frac{dx_0(s_{0,0})}{ds} = 0.00006216022389335293,\\
w_{0,0,1} &= \gamma_{0,0}\gamma_{0,0,1}\frac{dx_0(s_{0,0})}{ds} = 0.00006216022389335293.
\end{align*} 

This process would be repeated for the other intermediate quadrature points and other curves.
