# Supplementary material for: High-accuracy mesh-free quadrature for trimmed parametric surfaces and volumes
Source: arXiv:2101.06497 source file (2022-01-02)
Supplement: Supplementary file 3 [file appendixA_booleans.tex]

\section{Booleans of Rational Shapes}
\label{app:booleans}
Intersections, unions, and differences of rational shapes can be computed using the algorithm given in Section~\ref{sec:algorithm} by using \bezier\ intersection and reparametrization. 
An algorithm for computing parametrizations of Boolean combinations (i.e. unions, intersections, and differences) of regions defined by polynomial triangular Bernstein-\bezier\ elements is described in~\cite{hermes2018high}. We have adapted this algorithm to the rational case to help design some of the shapes for our empirical results in Section~\ref{sec:results}. Our approach combined with efficient intersection could be used to efficiently perform the integration necessary in immersogeometric analysis, field transfer between high-order meshes, and VOF field initialization, in which integrals over intersections between rational geometries must be computed.
