# Supplementary material for: High-accuracy mesh-free quadrature for trimmed parametric surfaces and volumes
Source: arXiv:2101.06497 source file (2022-01-02)
Supplement: Supplementary file 4 [file appendixB_NURBS.tex]

\section{NURBS}
\label{app:NURBS}

The algorithm described in Section~\ref{sec:algorithm} can easily be used on regions bounded by non-uniform rational basis splines (NURBS). Because NURBS can be decomposed exactly into rational \bezier\ curves, the algorithm only requires one extra step: \bezier\ extraction~\cite{borden2011isogeometric}, which converts a degree-$m$ NURBS curve into component degree-$m$ rational \bezier\ curves.  
